# Supplementary material for: Fault-Tolerant Hybrid-Parallel Training at Scale with Reliable and Efficient In-memory Checkpointing
Source: arXiv:2310.12670 source file (2024-08-19)
Supplement: Supplementary file 1 [file 1_appendix.tex]

\appendix
\section{Derivation of  Optimal Frequencies}
In our design, \name~run asynchronously to avoid interference with the pretraining processes introducing limited overhead for pretraining. The policy for determining the snapshotting and checkpointing frequencies, which we define as the interval $T_{sn}$ and $T_{ckpt}$ depends on the observed or theoretical Mean-Time-to-failure (MTTF) of the system.

In general, the optimal snapshot/ checkpoint interval $T_{save}$ \cite{maeng_cpr_2020} that minimize the total overhead $O_{total}$ can be obtained from
\begin{equation}
O_{total} = O_{save}\frac{T_{total}}{T_{save}}+O_{restart}T_{total}\lambda_{fail}\\
\end{equation}
where $O_{save}$ is the parameter saving overhead, $T_{total}$ is the overall training time, and $\lambda_{fail}$ is the average failure rate, i.e. reciprocal of MTTF. ${O_{restart}}$ is the restarting overhead. The first item refers to the saving overhead, and the second one is the restarting overhead, including average recomputations $T_{save}/2$, rescheduling overhead $T_{sch}$, and loading overhead $T_{load}$. Then we derive the optimal interval:
\begin{equation}
T_{save} = \sqrt{2 \frac{ O_{save}}{\lambda_{fail} }}
\end{equation},

In checkpoint-based fault tolerance, single-node failure results in the collapse of the entire computation, which makes the system failure rate equate to the single-node failure rate $\lambda_{nd\_fail}$: 
\begin{equation}
\lambda_{ck\_fail} = \lambda_{nd\_fail}
\end{equation}

In \name, only when more than one node fails in an $SG$ will we need to restart training from a previous checkpoint. This gives us failure rate $\lambda_{re\_fail}$ of \name~failing to restore parameters from CPU memory - that is when checkpoints are necessary:
\begin{equation}
\lambda_{re\_fail} = 1-(1-\lambda_{nd\_fail})^n - n\lambda_{nd\_fail}(1-\lambda_{nd\_fail})^{(n-1)}
\end{equation}

We denote $T_{comp}$ as the computation time, which comprises the sum of forward and backward time, i.e., $T_{comp}=T_{fwd}+T_{bwd}$. 
And $T_{ft}$ as the fault-tolerance overhead, including snapshotting overhead $T_{sn}$ or the checkpointing overhead $T_{ckpt}$. We have:

% \begin{equation}
% O_{save}= \left\{
% \begin{aligned}
% T_{ft}-T_{comp}, \quad T_{ft} > T_{comp} \\
% 0, \quad T_{ft}\leq T_{comp}
% \end{aligned}
% \right.
% \end{equation}

\begin{equation}
    O_{save}=\frac{1}{2}\left(|T_{ft}-T_{comp}| + T_{ft}-T_{comp}\right)
\end{equation}
\name~benchmarks user-defined training iterations and calculate the average snapshotting overhead $\bar O_{re\_save} $. $\lambda_{fail}$ could be empirically observed from average failure rates or attained from the server provider. Therefore, with $\lambda_{re\_fail}$ and $\bar O_{re\_save} $, \name~can automatically determine the snapshotting interval $T_{sn} = \sqrt{2 \frac{\bar O_{re\_save}}{\lambda_{re\_fail} }}$ that minimizes $O_{total}$ after benchmarking. We have the optimal snapshotting interval with \name~as $T_{re\_{sn}}$, and the  optimal  checkpointing interval without \name~as $T_{ckpt}$:
\begin{equation}
T_{re\_{sn}} = \sqrt{\frac{|T_{sn}-T_{comp}| + T_{sn}-T_{comp}}{\lambda_{nd\_fail} }}
\end{equation}

\begin{equation}
T_{ckpt} = \sqrt{\frac{|T_{ckpt}-T_{comp}| + T_{ckpt}-T_{comp}}{\lambda_{nd\_fail} }}
\end{equation}

As is shown in Figure \ref{fig:pipe}, checkpointing of \name~on SMP does not introduce additional overheads to training, we have  the  optimal checkpoint interval in \name~as:
\begin{equation}
T_{re\_{ckpt}} = \sqrt{\frac{|T_{sn}-T_{comp}| + T_{sn}-T_{comp}}{1-(1-\lambda_{nd\_fail})^n - n\lambda_{nd\_fail}(1-\lambda_{nd\_fail})^{(n-1)}}}
\end{equation}

The analysis provides an optimal solution for the fault-tolerance frequencies. In practice, the user could adjust the frequencies based on the practical need, e.g., increasing the frequency to improve the version control of the parameters; and decreasing the frequency if IO is too slow or the cloud storage is limited.
